# Supplementary material for: First-order methods for the convex hull membership problem
Source: arXiv:2111.07720 source file (2022-08-29)
Supplement: Supplementary file 1 [file appendix.tex]

\section{Appendix}
\label{append:pivoestrito}
In this appendix some demonstrations of facts that were used throughout the article will be presented.

\subsection{Triangle Algorithm}
Lemma for strict pivot characterization analogous to Lemma~\ref{lema:pivo}
\begin{lema}
 	Let $p_k \in \convA$, $v_j \in \mathcal{A}$ and $p \in \Rm$ be given. The following are equivalent:
 	\begin{listi}
 		\item $\norm{v_j-p}^2 \leq \norm{v_j-p_k}^2 - \norm{p_k-p}^2;$
 		\item $2v_j^T(p_k-p) \leq 2p^T(p_k-p);$
 		\item $(p_k-p)^T(v_j-p_k) \leq -\norm{p_k-p}^2$;
 		\item $(p_k-p)^T(v_j-p) \leq 0.$
 	\end{listi}
\end{lema}

\subsection{Numerical Experiments}

\subsubsection{Case (b)}
\label{append:case(b)}
In section~\ref{sec:caseb} considering the tolerance $\varepsilon=10^{-4}$ the algorithms TA and GT reached the maximum iteration. By increasing $\varepsilon$ to $10^{3}$ we choose the following results in relation to time:

\begin{figure}[!htpb]
\centering
	\begin{subfigure}[t]{.48\linewidth}
	\includegraphics[scale=0.5]{imagens/Casebpequeno1e-3.eps}
	\caption{}
	\end{subfigure}
	\begin{subfigure}[t]{.48\linewidth}
    \centering	
	\includegraphics[scale=0.5]{imagens/Casebgrande1e-3.eps}
	\caption{}
	\end{subfigure}
	\caption{Case (b). Running times (in seconds) for dimension $m=100$ and increasing $n$, the number of points in $\A$. }\label{fig:casec}
\end{figure}

\subsubsection{Estimative $D$ and $\Omega_C$ }
\label{append:DeOmega}
Let be $C= \conv{\tilde{A}}$ then 

\begin{equation} \label{eq:sistemafacPL}
\begin{aligned}  D \coloneqq \max \{ \| x - y \|\mid x,y \in C \} &\geq  \Big\|\left(\begin{array}{c}
0 \\
0 \\
1 \end{array}\right)- \left(\begin{array}{c}
-b \\
-N \\
1 \end{array}\right)\Big\| \geq N+1.
\end{aligned}
\end{equation}
Moreover $\bar{v}= (-b^T,-N,1)^T$ is a extreme point from $\conv{\tilde{A}}$ and an inequality that is not valid at this vertex is when $a_j= (0^T,0, -1)^T$ and  $b_j = 0$, then:
\begin{equation}
    \Omega_C \coloneqq \displaystyle \min_{v\in V,  \,i\in \{1,\ldots, m\}\mid b_i> a_i^T v}  \dfrac{b_i -  a_i^T v}{\|a_i\|} \leq \frac{b_j-a_j^T\bar{v}}{\norm{a_j}}= 1.
\end{equation}
